# Supplementary material for: ExPUNations: Augmenting Puns with Keywords and Explanations
Source: arXiv:2210.13513 source file (2022-10-24)
Supplement: Supplementary file 1 [file merged_keywords.tex]

\section{Statistics for aggregated keywords}
\label{app:aggregated}
